# Supplementary material for: Evaluating Robustness of Visual Representations for Object Assembly Task Requiring Spatio-Geometrical Reasoning
Source: arXiv:2310.09943 source file (2024-02-06)
Supplement: Supplementary file 1 [file methods.tex]

\section{Object Models}
\label{sec:object_models}
Every object model shares the same 8cm $\times$ 8cm $\times$ 8cm cubical base.
All extrusions are standardized to have a height of 2cm and all intrusions to a depth of 2.5cm, but the tolerance of the shapes parallel to the block face varies from 1-4mm.
For a more detailed look at the peg and hole models used in the task, Fig.~\ref{fig:dataset_example} shows an example of a plus-shaped peg and hole pair with relevant measurements of the intrusion and extrusion. In general, the intrusions on the ``hole'' models are slightly larger than the extrusions on the ``peg'' models to allow for some tolerance when fitting the two objects together. The figure also shows an example of 3D printed peg and hole models in the real world, which adhere to the exact same scale as the objects used in simulation.

\ku{In Fig.~\ref{fig:objects_45_deg_rotated}, we show the variation of objects with 45deg rotated extrusions.}

\begin{figure*}[h]
\centering
\includegraphics[width=\textwidth]{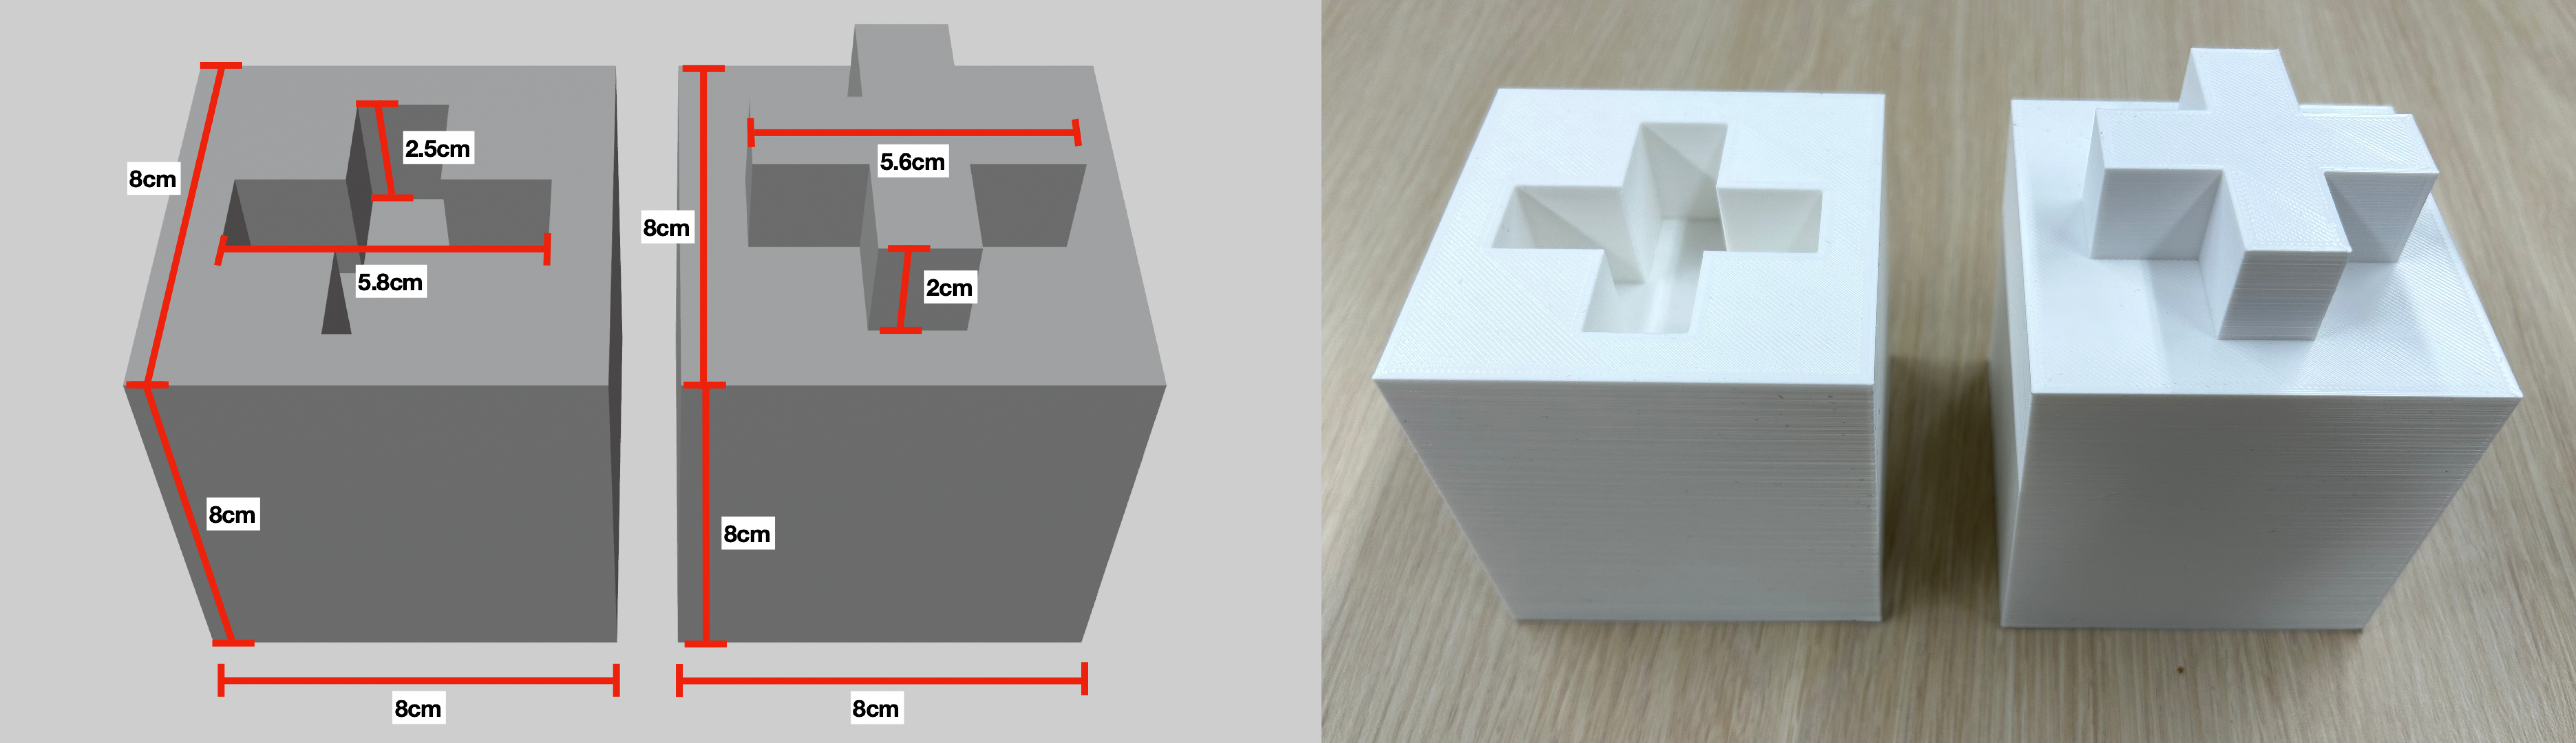}
\caption{An example object pair with a \textit{plus} intrusion and extrusion as 3D models with measurements (left) and in the real world (right).}
\label{fig:dataset_example}
\end{figure*}

\begin{figure*}[h]
\centering
\includegraphics[width=\textwidth]{images/objects_45_deg_rotated (1).png}
\caption{\ku{Objects with extrusions rotated by 45 degrees.}}
\label{fig:objects_45_deg_rotated}
\end{figure*}

\section{Training Hyperparameters}
\label{sec:hyperparameters}
All models had a MLP policy head of sizes $[1024, 1024, 18]$.
We use the original AveragePool and CLS-token outputs for downsampling the spatial dimensions of ResNet and ViT models, with the exception of \textit{\textbf{CLIP ResNet-50}} \cite{clip} which uses AttentionPool in the original implementation.
All models were trained with the Adam optimizer \cite{adam}, learning rate of 0.001, and batch size of 16, for 50000 steps.
All models were evaluated with 40 randomizations of the same seeds to ensure that models were evaluated on the same set of unseen randomizations over different points in training.
