# Supplementary material for: Evaluating Robustness of Visual Representations for Object Assembly Task Requiring Spatio-Geometrical Reasoning
Source: arXiv:2310.09943 source file (2024-02-06)
Supplement: Supplementary file 2 [file results.tex]

\section{Frozen Image Encoder vs. Fine-tuned Image Encoder}
\label{sec:frozen_unfrozen}
Unfreezing the perception modules for each of the pretrained networks during training has drastically different effects across each model.
Models such as the R3M and ImageNet ResNet-50 that had relatively poor performance when frozen had greatly improved performance with fine-tuned perception modules.
The most dramatic improvement can be seen in the ZTZR performance of the R3M ResNet-50 trained on 1000 episodes, with a jump from \textbf{0.225} frozen to \textbf{0.9} unfrozen.
The performance of the unfrozen ImageNet ResNet-50 in each case matches or surpasses the best performing frozen models, such as CLIP ResNet-50.
On the other hand, the success rates of both CLIP models completely collapse to \textbf{0} in all cases when unfrozen.
We hypothesize that the special attention-pooling mechanism that provided very strong representations during frozen inference makes the out-of-distribution fine-tuning untrainably unstable with our hyperparameters.
Even with the improvements in the pretrained models, in most cases they still fall short to the performances of the non-pretrained ResNet-18 and ResNet-50 models, with the ResNet-18 remaining the best-performing architecture.
This further reinforces our previous observation of ResNet-18 outperforming ResNet-50, showing that even though ResNet-50 has been extensively used for computer vision tasks, more compact or condensed representations might be better for policy learning.
\begin{figure*}[h!]
     \centering
     \includegraphics[width=\textwidth]{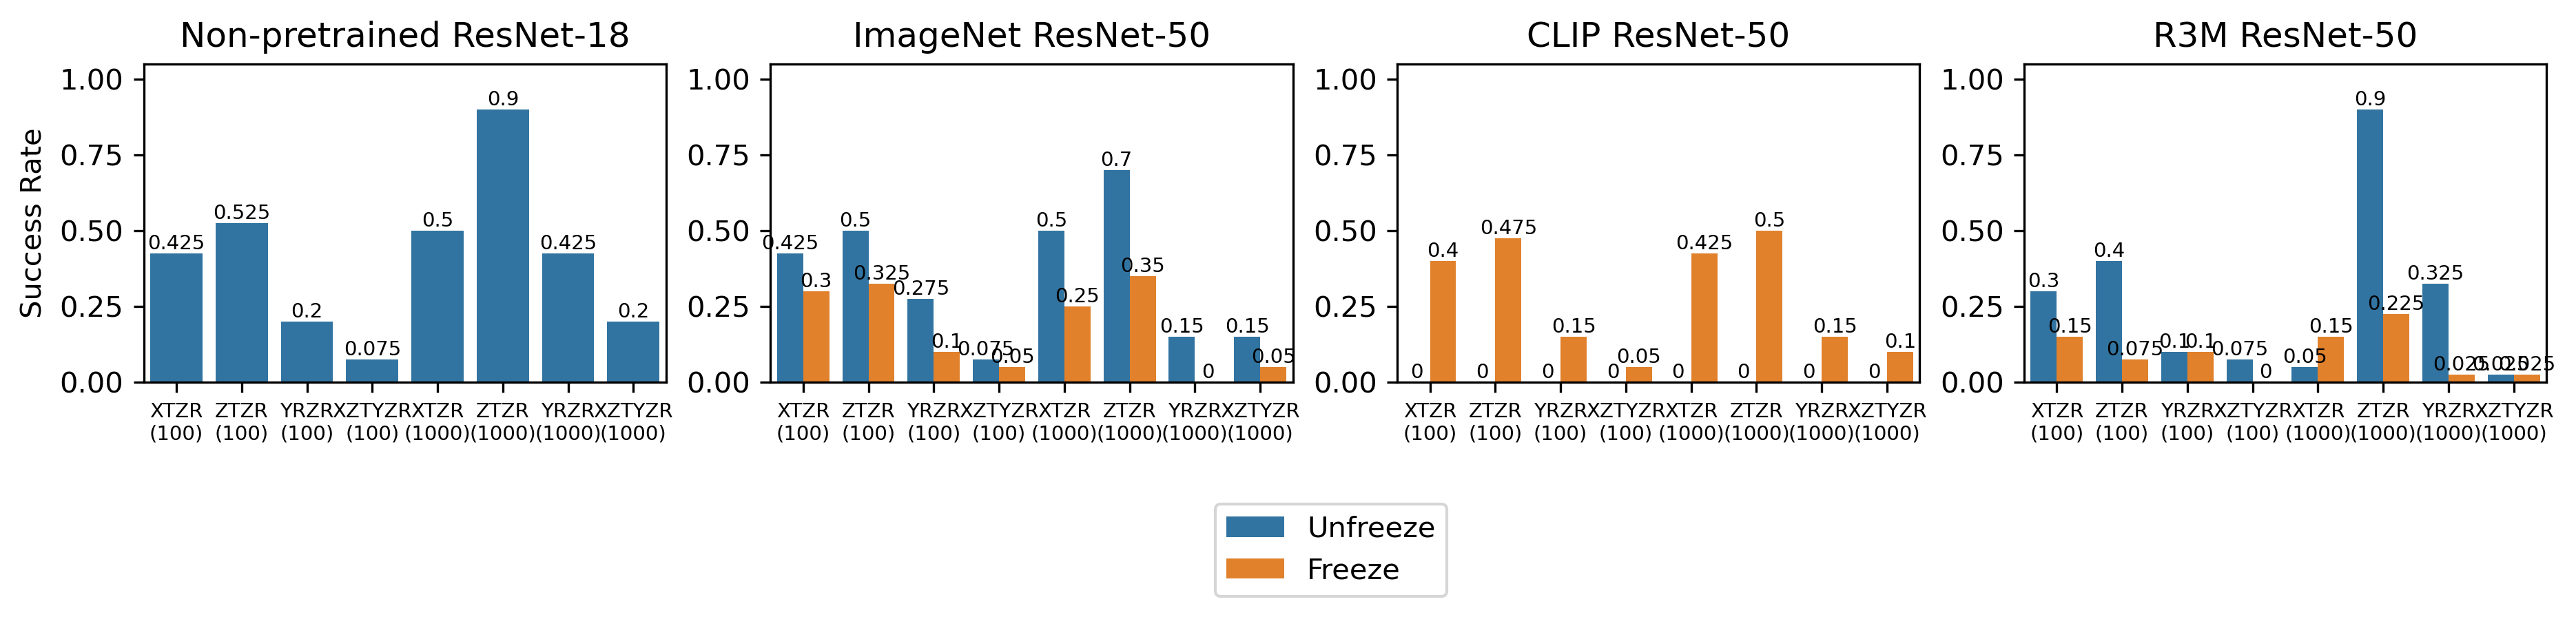}
     \includegraphics[width=\textwidth]{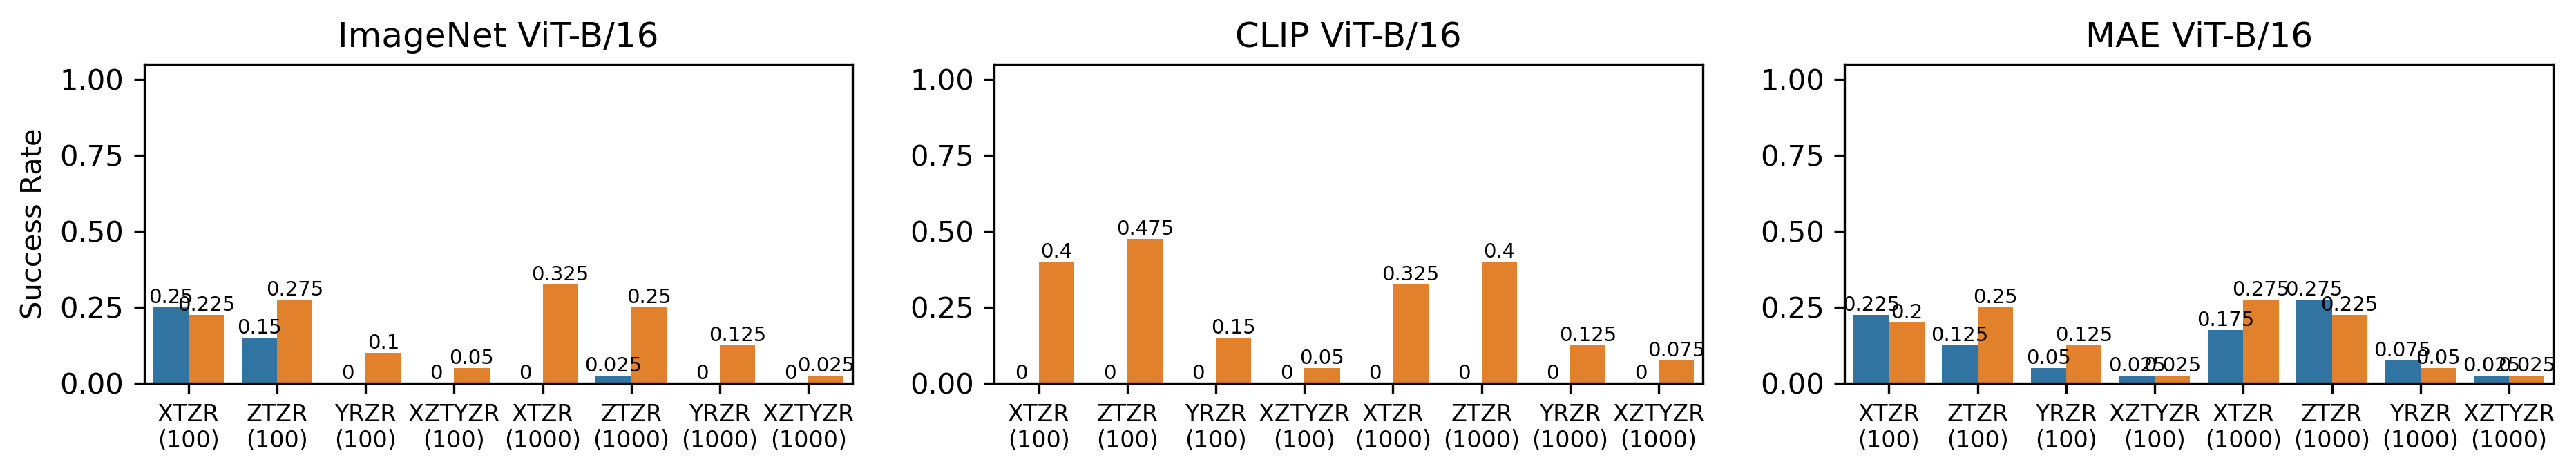}
     \caption{A comparison of the performances of all pretrained models with frozen versus unfrozen perception modules. Unfreezing the models lead to performance improvements for the ImageNet and R3M ResNet-50 architectures, and a complete collapse of both CLIP models. The unfrozen pretrained models were still unable to surpass the non-pretrained models.}
     \label{}
\end{figure*}

\section{Data Efficiency of Model Variations}
\label{sec:data_efficiency}
For non-pretrained models, the average performance increases drastically as the amount of data increases.
To specify, increasing from 100 episodes of demonstrations to 1000 episodes of demonstrations improves the average success rate by \textbf{0.27}, from \textbf{0.38} to \textbf{0.65} (see the bottom two rows of Fig.~\ref{fig:all_models_combo_variation}).
This improvement in performance is consistent although not as drastic when increasing from 1000 episodes to 10000 episodes, with the average success rate increasing by \textbf{0.05}, from \textbf{0.65} to \textbf{0.70}. 
As the vision encoders are fine-tuned, they get better at identifying the spatial information relevant for the task, improving success rates.
However, as we freeze pretrained vision encoders, those model variations rely solely on the MLP policy head for learning the trajectory.
We hypothesize that the variations with pretrained vision encoders do not improve with more data for two reasons: the MLP policy head is saturated with just 100 examples and the features from models trained on out-of-distribution data lack geometric-spatial information necessary to complete the task.

\begin{figure*}[h!]
     \centering
     \includegraphics[width=\textwidth]{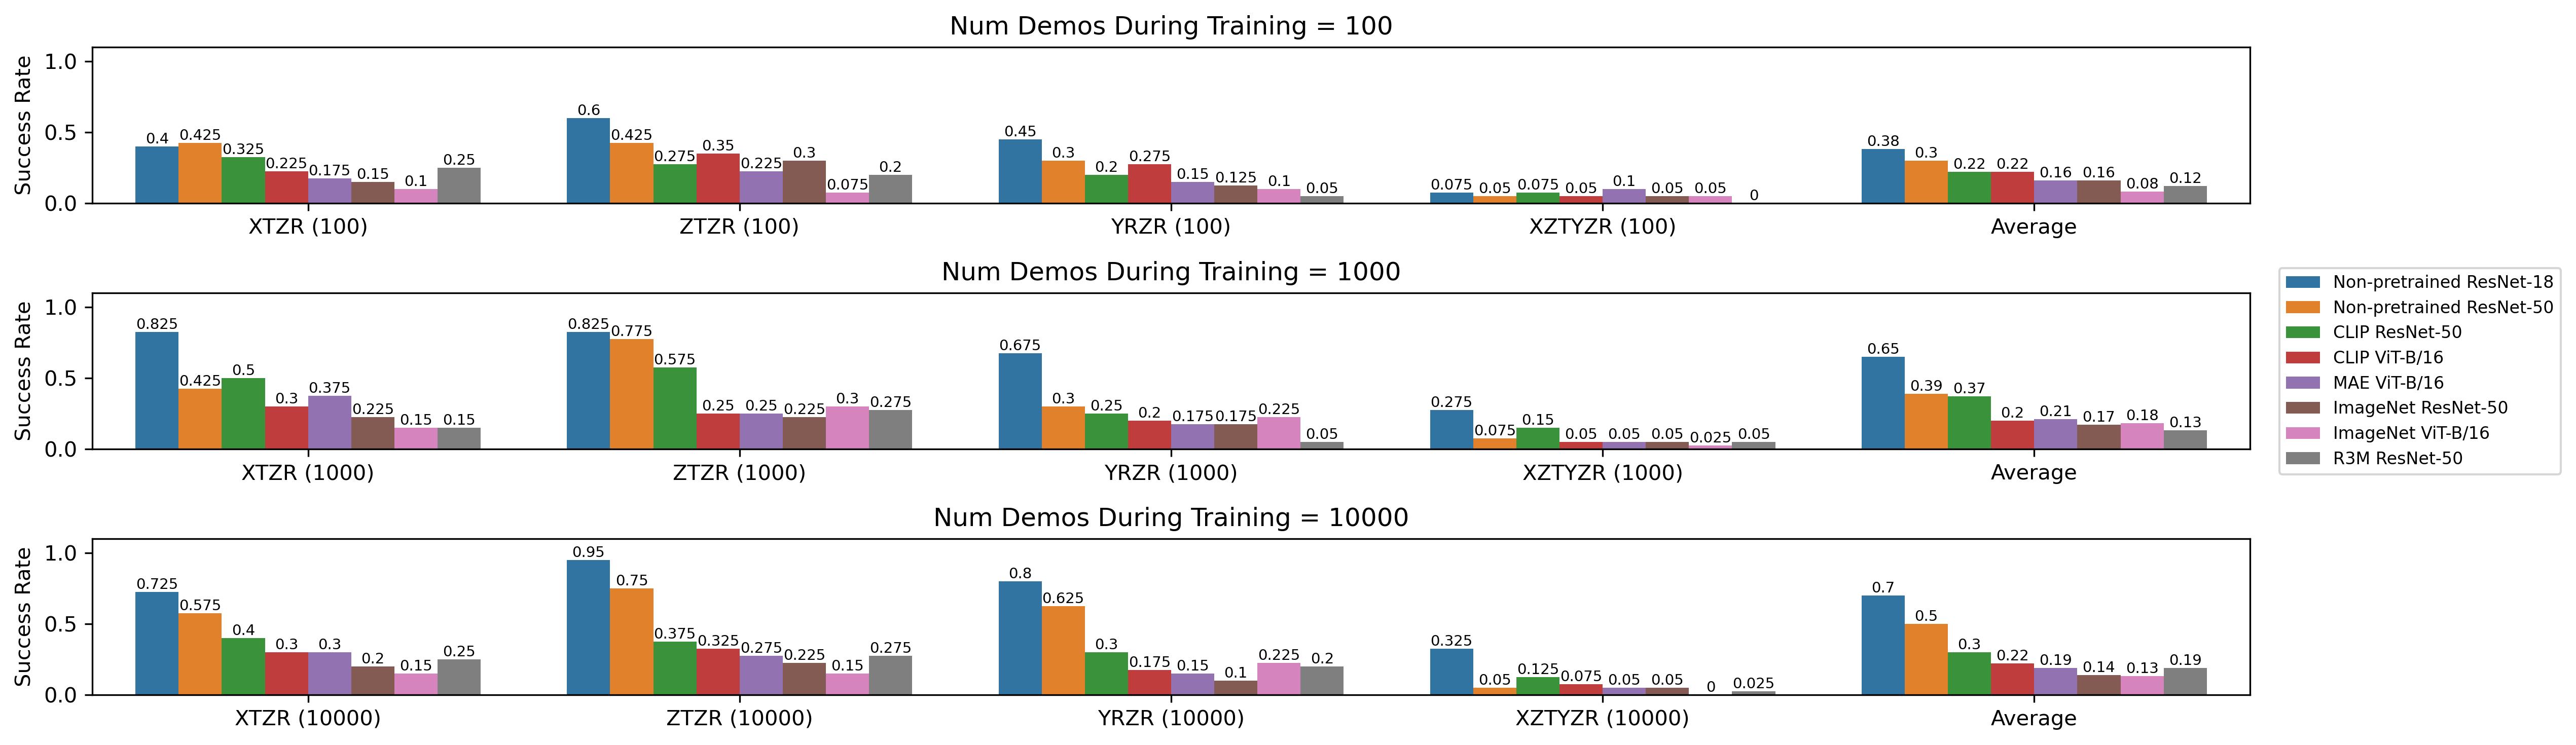}
     \caption{A comparison of all models on more complex task variants (i.e. rotations/translations along multiple axes).}% The added complexity to the task caused decreases in performance from one-variation tasks across all models trained on 100 episodes. When trained on more data, only the non-pretrained models saw general performance improvements.}
     \label{fig:all_models_combo_variation}
\end{figure*}

\section{Comparison on Specific Object Sets}
\label{sec:object_sets}
We compare the performance on different object sets by training models on \textit{\textbf{Order-all}} and evaluating them separately on 40 random initializations of \textit{\textbf{Order-1}}, \textit{\textbf{Order-2}}, \textit{\textbf{Order-4}}, and \textit{\textbf{45deg-Rotated}}.
We observe that \textit{\textbf{Order-1}} objects are hardest to learn as expected, since they have the most number of possible rotations.
To our surprise, however, we observe that \textit{\textbf{Order-4}} objects, which have 1 possible rotation and intuitively are the easiest to learn the policy on, do not perform the best for most task variations.
Upon closer inspection, we realized that policies are learned from easiest to hardest object sets.
Initially, the model learns to follow the general trajectory while ignoring any variations in the Z-rotation, achieving perfect accuracy for \textit{\textbf{Order-4}}.
Then, the second Z rotation is learned which is $90\degree$ apart from the default trajectory, improving results on \textit{\textbf{Order-2}}.
While this happens, the performance on \textit{\textbf{Order-4}} decreases, signifying a tradeoff between the performance on different object sets.
Similarly, as the model learns geometric reasoning on the most challenging \textit{\textbf{Order-1}} objects, the performance on \textit{\textbf{Order 4}} and \textit{\textbf{Order-2}} further degrades.
We hypothesize that this is due to (1) the multimodality of data where the possible variations of trajectories vary drastically depending on the object type and (2) the limited capacity of the vision encoder and the policy head.

\begin{figure*}[h!]
     \centering
     \includegraphics[width=0.7\textwidth]{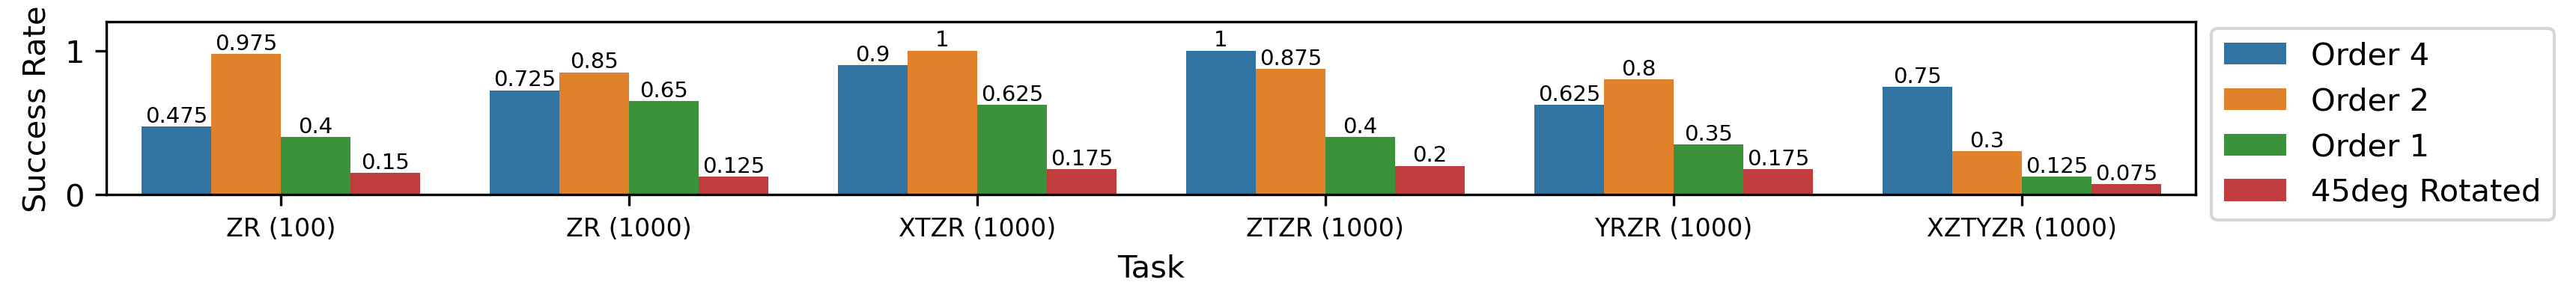}\includegraphics[width=0.25\textwidth]{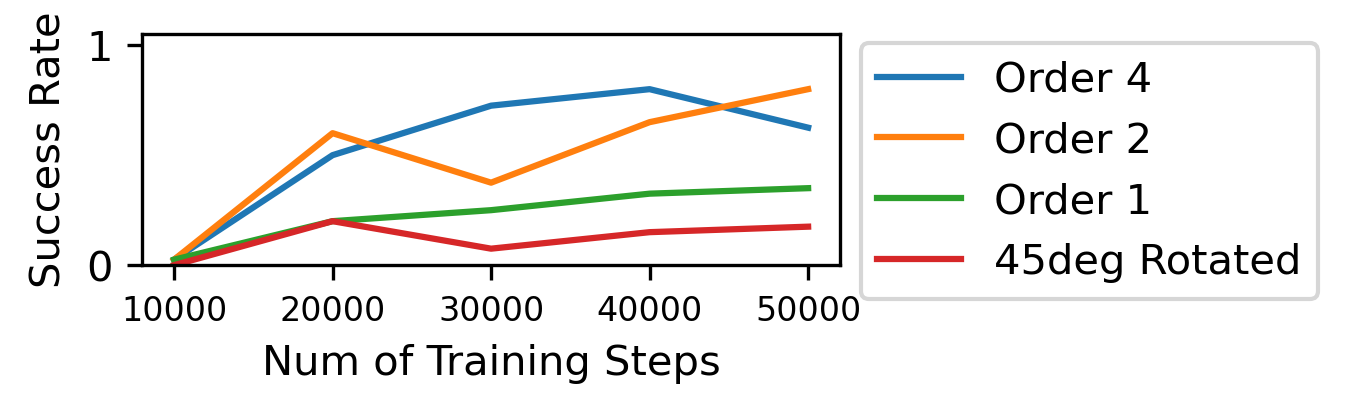}
     \caption{A comparison of all models evaluated on different sets of objects with a specific order of rotational symmetry, as well as a set of object pairs whose extrusions are rotated by 45$\degree$ (left), and a plot of success rates for each object set versus the number of training steps for \textbf{\textit{YRZR}} (right).}
     \label{fig:object_set_results}
\end{figure*}

\section{Importance of Wrist-view}
\label{sec:wrist_view}
We compare the performance of \textbf{\textit{Non-pretrained ResNet-18}} on \textbf{\textit{Wrist-view}} and \textbf{\textit{Top-view}}.
As expected, the addition of wrist-views improves results for most tasks in most data quantities, with greater amount of improvements for more challenging tasks and a higher quantity of data.
This phenomenon may be attributed to the usefulness of the extra signals provided by the wrist-views depending on the context: the robot may be able to reason better about the slight ablations in the rotations of the two cubes about the Y-axis with the added wrist-views since the top-view does not portray these variations as clearly.
The extra reasoning power would be a great benefit for YR variations but may only serve as noise for ZR variations, especially at the point in the task when the orientations of the intrusion and extrusion are already lined up.

\begin{figure*}[h!]
     \centering
     \includegraphics[width=\textwidth]{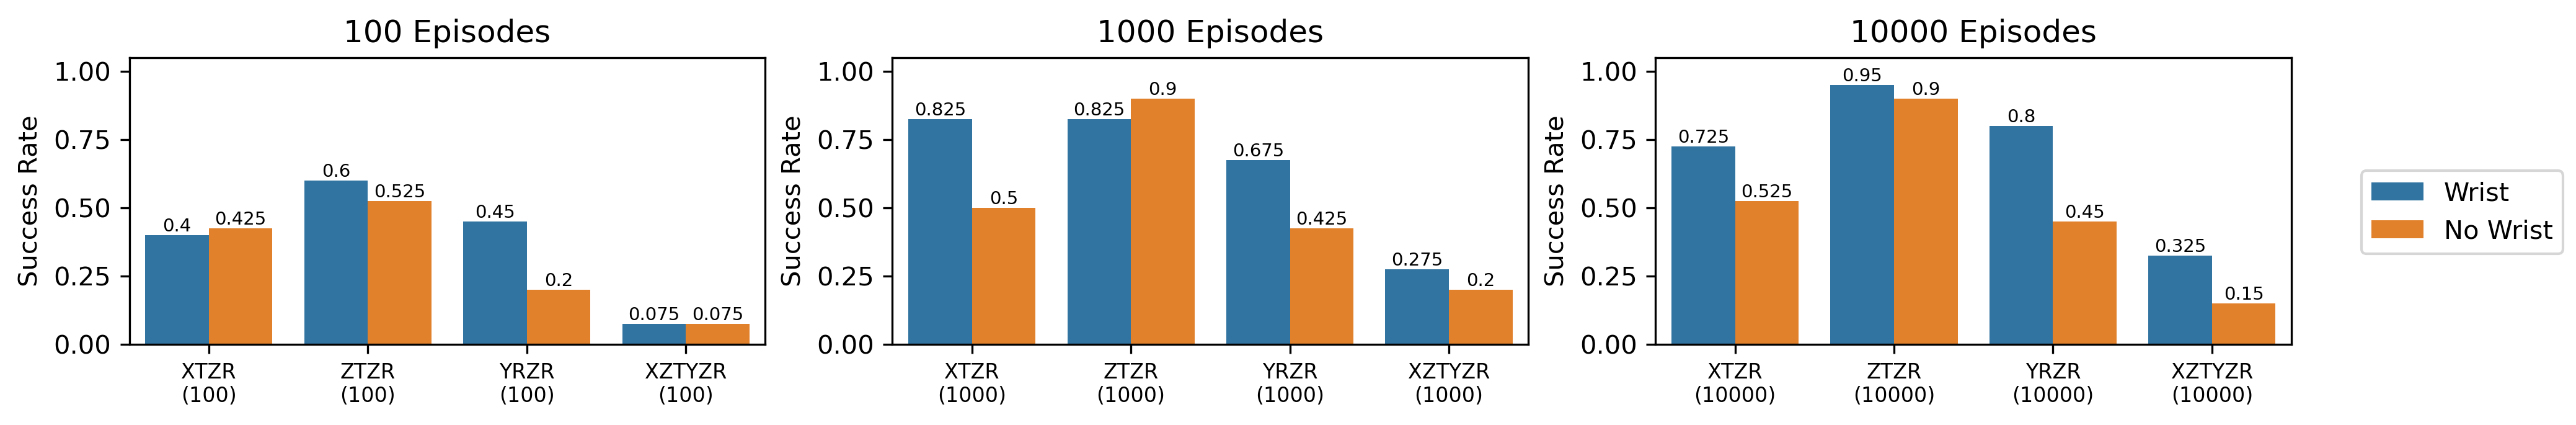}
     \caption{A comparison of performances for the non-pretrained ResNet-18 model when trained with wrist-views versus without. The added wrist-views lead to general improved performance across all variations that involved z-axis rotation.}
     \label{}
\end{figure*}

\color{blue}
\section{Comparison with SOTA BC Baseline. BC-RNN}
\label{sec:bcrnn}
\begin{table}[h!]
\centering
\resizebox{\textwidth}{!}{%
\begin{tabular}{|l|l|l|l|l|l|l|l|l|}
\hline
Models            & XT (1000) & ZT (1000) & YR (1000) & ZR (1000)      & XTZR (1000) & ZTZR (1000) & YRZR (1000) & XZTYZR (1000) \\ \hline
resnet18 BC-MLP   & 1         & 1         & 1         & 0.775          & 0.825       & 0.825       & 0.675       & 0.275         \\ \hline
resnet18 BC-RNN   & 1         & 1         & 1         & \textbf{0}     & 0.525       & 0.3         & 0.35        & 0.075         \\ \hline
clip50 BC-MLP     & 1         & 1         & 0.975     & 0.625          & 0.5         & 0.575       & 0.25        & 0.15          \\ \hline
clip50 BC-RNN     & 1         & 1         & 0.525     & \textbf{0.075} & 0.3         & 0.325       & 0.15        & 0.2           \\ \hline
clip\_base BC-MLP & 1         & 1         & 0.9       & 0.575          & 0.3         & 0.25        & 0.2         & 0.05          \\ \hline
clip\_base BC-RNN & 0.775     & 1         & 0.45      & \textbf{0}     & 0.15        & 0.35        & 0.025       & 0.025         \\ \hline
\end{tabular}}
\bigskip
 \caption{\ku{Performance of Non-pretrained ResNet-18, CLIP ResNet-50, and CLIP ViT-Base with MLP vs LSTM action decoders.}}
\end{table}
\textbf{Details of the Experiment:} We compare our original setup, BC-MLP with various image encoders, against BC-RNN \cite{robomimic}, a popular SOTA BC baseline that is shown to improve performance over BC-MLP. Instead of a MLP of layer sizes [1024, 1024, 18] on top of the image encoder, BC-RNN has two LSTM layers of hidden sizes [1024, 1024] and output size 18 that fuses image embeddings and proprioception from 10 most recent time frames as implemented in the original paper  \cite{robomimic}. The tabulated results show success rates evaluated over 40 rollouts. These models are all trained on 1000 demonstrations with proprioception and 3 views (top + 2 wrist cameras).

\textbf{Observation from the Experiment:} Contrary to our expectations, we observe that the performance is worse for BC-RNN on all tasks and models we ran these experiments on: Non-pretrained ResNet-18, CLIP ResNet-50, and CLIP ViT-base. We hypothesize that BC-RNN cannot use the history as well as it performed in the Robomimic work  \cite{robomimic}, because BC-RNN performs better on longer tasks while our tasks are relatively short. To be more specific, the 5 tasks in the RoboMimic paper have average episode lengths of 48 (Lift), 116 (Can), 151 (Square), 469 (Transport), and 480 (Tool Hang), where the performance of BC-RNN improved for only the longer three tasks. In comparison to their longer tasks, our tasks average around 10 to 40 frames, depending on the task variation. However, in the BC-RNN versions, we still observe similar trends between the visual encoders, as the performance is highest for Non-pretrained ResNet-18, followed by CLIP ResNet-50, followed by CLIP ViT-base.

\section{Statistical Analysis of Performance on Specific Objects}
\label{sec:stats}

\begin{table}[]
\begin{tabular}{|l|l|l|l|l|}
\hline
                    & XTZR (1000)  & ZTZR (1000)  & YZR (1000)   & XZTYZR (1000) \\ \hline
resnet\_18 circle   & 0.850+-0.066 & 1.000+-0     & 0.833+-0.052 & 0.425+-0.066  \\ \hline
resnet\_18 plus     & 0.933+-0.038 & 1.000+-0     & 0.767+-0.014 & 0.375+-0.043  \\ \hline
resnet\_18 minus    & 0.800+-0.025 & 0.975+-0     & 0.442+-0.101 & 0.333+-0.101  \\ \hline
resnet\_18 diamond  & 0.767+-0.063 & 1.000+-0     & 0.325+-0.075 & 0.342+-0.076  \\ \hline
resnet\_18 hexagon  & 0.708+-0.076 & 1.000+-0     & 0.383+-0.08  & 0.300+-0.075  \\ \hline
resnet\_18 u        & 0.367+-0.076 & 0.542+-0.058 & 0.117+-0.058 & 0.167+-0.029  \\ \hline
resnet\_18 pentagon & 0.342+-0.095 & 0.558+-0.038 & 0.100+-0.066 & 0.183+-0.072  \\ \hline
resnet\_18 arrow    & 0.383+-0.072 & 0.658+-0.076 & 0.183+-0.029 & 0.167+-0.052  \\ \hline
resnet\_18 key      & 0.375+-0.066 & 0.658+-0.076 & 0.167+-0.038 & 0.192+-0.052  \\ \hline
resnet\_18 all      & 0.614+-0.02  & 0.821+-0.025 & 0.369+-0.048 & 0.276+-0.033  \\ \hline
\end{tabular}
\bigskip
 \caption{\ku{Performance of Non-pretrained ResNet-18 on each object. Mean and standard deviations over 3 different evaluations of 40 randomized rollouts.}}
\end{table}

\ku{\textbf{Details of the Experiment:} We provide a more fine-grained evaluation of our best model (Non-pretrained ResNet-18) by running 3 different evaluation runs of 40 randomized episodes and reporting the mean and standard deviation over the 3 runs. \textit{resnet\_18 all} denotes the average of all evaluation runs above (total 360 episodes). These models are trained on 1000 demonstrations, which includes all shapes, with proprioception and 3 views (top + 2 wrist cameras).

\textbf{Observation from the Experiment:} We observe that the success rates are mostly consistent when evaluated on a completely new set of 40 randomized episodes, with a standard deviation ranging around 0.05. We observe that while the success rate of rotation groups (Order-4: circle and plus, Order-2: minus, diamond, and hexagon, Order-1: u, pentagon, and arrow) decline consistently from more to fewer degrees of symmetry. However, there is no clear trend in the order of performance for objects inside each group.}

\section{Real World Experiments}
\label{sec:real_world}

\begin{table}[h!]
\resizebox{\textwidth}{!}{%
\begin{tabular}{|l|l|l|l|l|l|l|l|l|}
\hline
Shape & XT (30) & ZT (30) & YR (30) & ZR (30) & XTZR (30) & ZTZR (30) & YRZR (30) & XZTYZR (30) \\ \hline
plus  & 0.3     & 0.2     & 0.2     & 0.9     & 0.2       & 0.5       & 0.1       & 0.0         \\ \hline
minus & 0.5     & 0.2     & 0.1     & 0.5     & 0.2       & 0.6       & 0.0       & 0.0         \\ \hline
key   & 0.3     & 0.0     & 0.2     & 0.3     & 0.1       & 0.3       & 0.1       & 0.0         \\ \hline
\end{tabular}}
\bigskip
 \caption{\ku{Performance of Non-pretrained ResNet-18 in the real world setup, when a single model was trained for all objects.}}
\label{Tab:one_for_all_shapes}
\end{table}

\begin{table}[h!]
\resizebox{\textwidth}{!}{%
\begin{tabular}{|l|l|l|l|l|l|l|l|l|}
\hline
Shape & XT (10) & ZT (10) & YR (10) & ZR (10) & XTZR (10) & ZTZR (10) & YRZR (10) & XZTYZR (10) \\ \hline
plus  & 0.9     & 1.0     & 0.7     & 1.0     & 0.6       & 0.7       & 0.2       & 0.3         \\ \hline
minus & 1.0     & 1.0     & 1.0     & 0.7     & 0.4       & 0.5       & 0.3       & 0.0         \\ \hline
key   & 1.0     & 1.0     & 0.5     & 0.0     & 0.0       & 0.3       & 0.0       & 0.1         \\ \hline
\end{tabular}
}
\bigskip
 \caption{\ku{Performance of Non-pretrained ResNet-18 in the real world setup, when separate models were trained for each object.}}
\label{Tab:one_per_shape}
\end{table}

\textbf{Details of the Experiment:} We conduct real world experiments to verify if (1) our observations from the simulation experiments are consistent with the real world (2) our setup can generalize with fewer demonstrations on the real robot. We experiment with a setup that is more similar to our simulation setup by training a single model to generalize over all the shapes (Table ~\ref{Tab:one_for_all_shapes} one model for all shapes). We calculate the success rates by counting "smooth insertions," which does not include forcing the objects together such that objects slip into each other even when they are not aligned. In other words, we do not count unintended insertions that did not properly align the objects towards success. Additionally, we also experiment with a setup that has one model per shape (Table ~\ref{Tab:one_per_shape}).

\textbf{Observation from the Experiment:} We observe that one model for all shapes (Table ~\ref{Tab:one_for_all_shapes}) perform worse than models trained and evaluated in simulation, because of fewer number of demonstrations in the real world. In this setup, we were not able to draw conclusive observations on the exact trend of performance, due to high variance in success rates likely induced from limited number of train demonstrations (30 vs. 100/1000/10000) and evaluation runs (10 vs. 40). It is also worth noting that the real world setup does not have wrist cameras, adding to the performance drop compared to simulated experiments. In are additional experiments where we train one model per shape (Table ~\ref{Tab:one_per_shape}), we notice considerable improvements in success rates, suggesting that more demonstrations are needed to generalize over multiple shapes. However, the general trend of performance is consistent with our simulation setup: (a) objects with more degrees of symmetry perform better (b) tasks with simpler variations perform better than combinations (e.g. ZR performs better than XTZR, ZTZR, YRZR, and XZTYZR for all shapes except the key).

\section{Comparison of Models with and without Proprioception}
\label{sec:prop}

\begin{table}[h!]
\resizebox{\textwidth}{!}{%
\begin{tabular}{|l|l|l|l|l|l|l|l|l|}
\hline
                    & XT (1000)      & ZT (1000)      & YR (1000)      & ZR (1000)      & XTZR (1000)    & ZTZR (1000)    & YRZR (1000)    & XZTYZR (1000)  \\ \hline
resnet18 with\_prop & 1              & 1              & 1              & 0.775          & \textbf{0.825} & \textbf{0.825} & \textbf{0.675} & \textbf{0.275} \\ \hline
resnet18 no\_prop   & 1              & 1              & 1              & 0.675          & 0.4            & 0.0            & \textbf{0.525} & 0.125          \\ \hline
clip50 with\_prop   & \textbf{1}     & \textbf{1}     & \textbf{0.7}   & \textbf{0.675} & \textbf{0.425} & \textbf{0.5}   & \textbf{0.15}  & \textbf{0.1}   \\ \hline
clip50 no\_prop     & 1              & 1              & 0.675          & 0.275          & 0.175          & 0.075          & 0.075          & 0.1            \\ \hline
r3m50 with\_prop    & \textbf{0.975} & \textbf{0.875} & \textbf{0.525} & \textbf{0.275} & \textbf{0.15}  & \textbf{0.225} & \textbf{0.025} & \textbf{0.025} \\ \hline
r3m50 no\_prop      & 0.2            & 0.775          & 0.45           & 0.025          & 0              & 0.025          & 0.05           & 0.15           \\ \hline
\end{tabular}}
\bigskip
 \caption{\ku{Performance of Non-pretrained ResNet-18, CLIP ResNet-50, and R3M ResNet-50 with and without proprioception.}}
\end{table}

\textbf{Details of the Experiment:} For Non-pretrained ResNet-18, CLIP ResNet-50, and R3M ResNet-50, we train new models without proprioception and compare the success rates over 40 rollouts. The only difference is in the input dimension of the action decoder: with\_prop has the current end effector pose concatenated to the image embeddings while no\_prop has just the image embeddings. Note that all other experiments from the paper are done with proprioception. These models are trained on 1000 demonstrations, which includes all shapes, and 3 views (top + 2 wrist cameras).
\textbf{Observation from the Experiment:} We observe that (1) proprioception is crucial for learning task variations with Z rotation and (2) proprioception reduces variance in models with lower-performing visual encoders (R3M ResNet-50). We hypothesize that the policy network benefits from explicitly knowing the robot's current state to accurately step toward the task goal. While in theory, the model can induce the current state of the object from images, we observe that explicitly stating the current state yields better results. Benefits from this explicit signaling is most clear when there are other perturbations along with Z rotation (XTZR, ZTZR, YRZR, XZTYZR).

\section{Colored vs. Original Objects in Simulation}
\label{sec:colored}

\begin{table}[h!]
\resizebox{\textwidth}{!}{%
\begin{tabular}{|l|l|l|l|l|l|l|l|l|}
\hline
 & XT (1000) & ZT (1000) & YR (1000) & ZR (1000) & XTZR (1000) & ZTZR (1000) & YRZR (1000) & XZTYZR (1000) \\ \hline
resnet18 colored & 1 & 1 & 1 & 0.975 & 0.525 & 0.825 & 0.4 & 0.325 \\ \hline
resnet18 original & 1 & 1 & 1 & 0.775 & 0.825 & 0.825 & 0.675 & 0.275 \\ \hline
clip50 colored & 0.95 & 0.95 & 0.925 & 0.175 & 0.35 & 0.25 & 0.15 & 0.125 \\ \hline
clip50 original & 1 & 1 & 0.975 & 0.625 & 0.5 & 0.575 & 0.25 & 0.15 \\ \hline
\end{tabular}}

\bigskip
 \caption{\ku{Performance of Non-pretrained ResNet-18 and CLIP ResNet-50 with original vs. colored objects.}}
\end{table}

\begin{figure*}[h!]
     \centering
     \includegraphics[width=.4\textwidth]{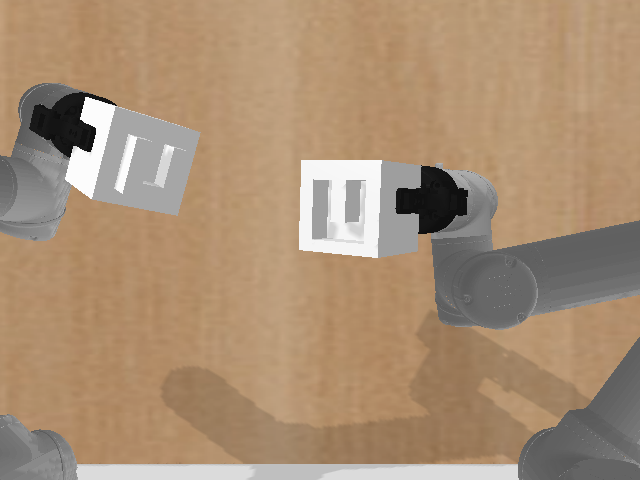}
     \includegraphics[width=.4\textwidth]{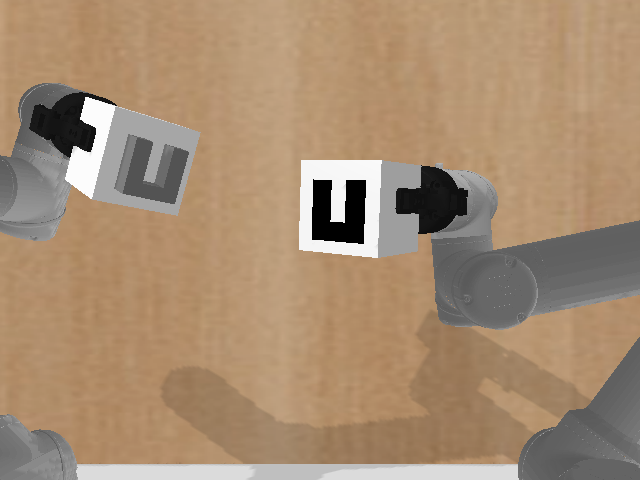}
     \caption{\ku{Examples of initial episode setup with original object (left) vs colored object (right).}}
     \label{}
\end{figure*}

\textbf{Details of the Experiment:} We compare the performance of models trained on the  colored objects with more contrast between the base and the extrusion (shown in figures below). We train and evaluate Non-pretrained ResNet-18 and CLIP ResNet-50 using 1000 demonstrations of each task variation.

\textbf{Observation from the Experiment:} To our surprise, we observe that performance of models trained with colored objects are comparable but not better than models trained with original objects. For example, the model trained on colored ZR performs better than original, but the model trained on colored XTZR performs worse than original. There is not a clear trend on which tasks the models trained on colored objects perform well.

\color{black}
